# Supplementary material for: $Z^*$: Zero-shot Style Transfer via Attention Rearrangement
Source: arXiv:2311.16491 source file (2023-11-25)
Supplement: Supplementary file 4 [file fig_supp_noise.tex]

\begin{figure*}%[t]
\setlength{\abovecaptionskip}{2mm}
\centering
\includegraphics[width=\textwidth]{image/noise}
\caption{Comparisons of model robustness with ArtFlow. We visualize the impact of adding a small perturbation $\Delta$ following a Gaussian distribution on the stylized images in the \engordnumber{4} and \engordnumber{7} columns.
}
\label{fig:noise}
\end{figure*}
