# Supplementary material for: $Z^*$: Zero-shot Style Transfer via Attention Rearrangement
Source: arXiv:2311.16491 source file (2023-11-25)
Supplement: Supplementary file 6 [file tab_supp_progressive.tex]

\begin{table}%[!h]
\small
\setlength\tabcolsep{2.5pt}
\centering
\begin{tabular}{c|c|c}
\toprule
&Single-layer &Ours (multi-layer)  \\
\midrule
$\contentloss$ $\downarrow$ & 1.94& \textbf{1.91} \\
$\styleloss$ $\downarrow$ & 2.38 & \textbf{1.47}  \\
\bottomrule
\end{tabular}
\vspace{-5pt}
\caption{Quantitative evaluation of progressive generation.}
\label{tab:loss1}
\end{table}
